# Supplementary material for: Classical route to quantum chaotic motions
Source: arXiv:2005.07714 ancillary file (2020-05-15)
Supplement: Supplementary file 1 [file supplementary_material.pdf]

# Supplementary material to "Classical route to quantum chaotic motions"

Nan Yang,[1,2,*] Xuedong Hu,[3,1] Yong-Chun Liu,[4] Ting Yu,[2] and Franco Nori[1,5]

[1] *Theoretical Quantum Physics Laboratory, RIKEN, Saitama, 351-0198, Japan*

[2] *Center for Quantum Science and Engineering, and Department of Physics, Stevens Institute of Technology, Hoboken, New Jersey 07030, USA*

[3] *Department of Physics, University at Buffalo, SUNY, Buffalo, New York 14260-1500, USA*

[4] *State Key Laboratory of Low-Dimensional Quantum Physics, Department of Physics, Frontier Science Center for Quantum Information, Collaborative Innovation Center of Quantum Matter, Tsinghua University, Beijing, 100084, China*

[5] *Physics Department, The University of Michigan, Ann Arbor, Michigan 48109-1040, USA*

(Dated: March 27, 2020)

This supplement provides supporting materials to the main text on the following topics: (i) The equations of motion for the setup in configuration I; (ii) The dynamics of the quantum mechanical resonator for different classical inputs in the setup of configuration I; (iii) The dynamics of the quantum cavity for different classical inputs in the setup of configuration II; (iv) The nonlinearity of closed quantum systems in configuration II.

## i. THE EQUATIONS OF MOTION FOR THE SETUP IN CONFIGURATION I.

In configuration I, the quantum chaotic motion is studied by the standard deviations $\sigma_x$ of a quantum harmonic oscillator. The chaos encoded in the standard deviations $\sigma_x$ can be decoded by the generalized quantum orbit, i.e., $\sigma_x(t)$ is embedded into a high dimensional space and reconstructed as a chaotic attractor. Physically speaking, this quantum chaotic motion refers to a chaotic vibration of the quantum wave packet.

The setup is shown in Fig. 1, which can be divided into a classical and a quantum parts, and chaos is transferred from the classical to the quantum components. Here, the quantum part includes a quantum cavity $\hat{a}_q$ and a quantum mechanical resonator $\hat{b}_q$. While, the classical part consists of an optomechanical resonator $(\hat{a}_c, \hat{b}_c)$ as the chaos generator and an optical cavity $\hat{a}_1$ to import chaos into the quantum mechanical mode $\hat{b}_q$. It is known that the location of a mechanical membrane in a cavity determines the optical-mechanical coupling types. Here, the mechanical membrane $\hat{b}_q$ is placed at an antinode of the cavity $\hat{a}_1$ to create a quadratic coupling, and at a node of the quantum cavity $\hat{a}_q$ for a linear coupling.

The free Hamiltonian of the total system is written as

$$\begin{aligned} H =&\Delta_1\hat{a}_1^\dagger\hat{a}_1 + \frac{1}{2}g_1\hat{a}_1^\dagger\hat{a}_1(\hat{b}_q^\dagger+\hat{b}_q)^2 + \Delta_q\hat{a}_q^\dagger\hat{a}_q + g_q\hat{a}_q^\dagger\hat{a}_q(\hat{b}_q^\dagger+\hat{b}_q) + \varepsilon_q(\hat{a}_q^\dagger+\hat{a}_q) + \Omega_q\hat{b}_q^\dagger\hat{b}_q \\ &+ \Delta_c\hat{a}_c^\dagger\hat{a}_c + g_c\hat{a}_c\hat{a}_c^\dagger(\hat{b}_c^\dagger+\hat{b}_c) + \Omega_c\hat{b}_c^\dagger\hat{b}_c + \varepsilon_c(\hat{a}_c^\dagger+\hat{a}_c), \end{aligned} \tag{1}$$

where $\Delta_j = \omega_j - \omega_{j,d}$ is the detuning between the resonant frequency $\omega_j$ and the external driving $\omega_{j,d}$ of the cavity mode $\hat{a}_j$ for $j = 1, q, c$; and its driving strength is denoted by $\varepsilon_j$. Here, the resonant frequency and the damping rate of the mechanical mode $\hat{b}_q$ ($\hat{b}_c$) are $\Omega_q$ ($\Omega_c$) and $\Gamma_q$ ($\Gamma_c$), respectively; $g_q$ ($g_1$) represents the coupling strength between the cavity mode $\hat{a}_q$ ($\hat{a}_1$) and the quantum mechanical resonator $\hat{b}_q$, while $g_c$ is the coupling strength between the classical cavity mode $\hat{a}_c$ and mechanical resonator $\hat{b}_c$.

---

*Electronic address: nyang.hust@gmail.com

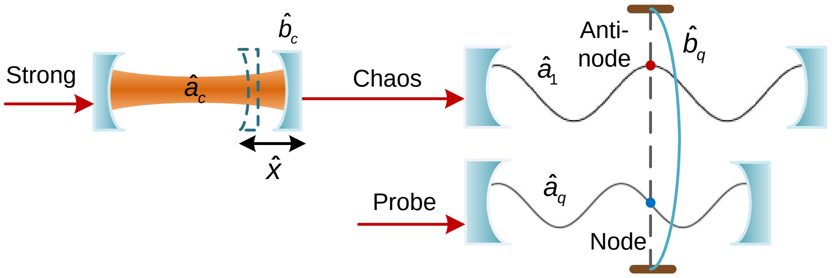


FIG. 1: (color online) Schematic diagram of an optomechanical setup for quantum chaos in configuration I.

### A. The equations of motion of the classical parts.

First, we consider the classical part ($\hat{a}_c$, $\hat{b}_c$, $\hat{a}_1$). The optomechanical resonator ($\hat{a}_c$, $\hat{b}_c$) is strongly driven to a chaotic state and then inputs the chaotic signal into the cavity mode $\hat{a}_1$. Their Langevin equations are given by

$$\dot{\hat{a}}_1 = -i\Delta_1\hat{a}_1 - \frac{\gamma_1}{2}\hat{a}_1 - \frac{i}{2}g_1\hat{a}_1(\hat{b}_q^\dagger + \hat{b}_q)^2 + \varepsilon_1 - \sqrt{\gamma_1\gamma_c}\,\hat{a}_c - \sqrt{\gamma_1}\hat{a}_{1,\text{in}} \tag{2a}$$

$$\dot{\hat{a}}_c = -i\Delta_c\hat{a}_c - ig_c\hat{a}_c(\hat{b}_c^\dagger + \hat{b}_c) - \frac{\gamma_c}{2}\hat{a}_c + \varepsilon_c - \sqrt{\gamma_c}\,\hat{a}_{c,\text{in}} \tag{2b}$$

$$\dot{\hat{b}}_c = -i\Omega_c\hat{b}_c - ig_c\hat{a}_c^\dagger\hat{a}_c - \frac{\Gamma_c}{2}\hat{b}_c - \sqrt{\Gamma_c}\,\hat{b}_{c,\text{in}} \tag{2c}$$

where $\gamma_j$ and $\hat{a}_{j,\text{in}}$ are the damping rate and the input of the optical cavity $\hat{a}_j$, for $j = 1, q, c$; while $\hat{b}_{\text{in}}$ ($\hat{b}_{c,\text{in}}$) and $\Gamma_q$ ($\Gamma_c$) are the input and the damping rate of the mechanical mode $\hat{b}_q$ ($\hat{b}_c$). Here, the effect of the quantum mechanical membrane $\hat{b}_q$ on the cavity mode $\hat{a}_1$ can be omitted, as it is comparably small.

In the strong-driving regime, the optomechanical system ($\hat{a}_c$, $\hat{b}_c$) and the cavity $\hat{a}_1$ can be treated classically. Therefore, their operators are replaced with the classical mean values: $\alpha_1 = \langle\hat{a}_1\rangle$, $\alpha_c = \langle\hat{a}_c\rangle$, and $\beta_c = \langle\hat{b}_c\rangle$. Then, from Eq.(2), we have the equations of motion for the classical parts

$$\dot{\alpha}_1 = -i\Delta_1\alpha_1 - \frac{\gamma_1}{2}\alpha_1 - \sqrt{\gamma_1\gamma_c}\alpha_c\ , \tag{3a}$$

$$\dot{\alpha}_c = -i\Delta_c\alpha_c - \frac{\gamma_c}{2}\alpha_c - ig_c\alpha_c(\beta_c + \beta_c^*) + \varepsilon_c\ , \tag{3b}$$

$$\dot{\beta}_c = \left(-i\Omega_c - \frac{\Gamma_c}{2}\right)\beta_c - ig_c|\alpha_c|^2\ . \tag{3c}$$

Here, the cavity mode $\alpha_1$ links both the classical and quantum parts together. The chaos generated by the optomechanical system ($\alpha_c$, $\beta_c$), is thus transferred into the quantum mechanical resonator $\hat{b}_q$.

### B. The equations of motion of the quantum part.

The quantum part of this setup includes the quantum mechanical resonator $\hat{b}_q$ and the quantum cavity $\hat{a}_q$. Since the classical part ($\hat{a}_c$, $\hat{b}_c$, and $\hat{a}_1$) can be treated classically, we have the reduced Hamiltonian

$$H_{\text{eff}} = \Delta_q\hat{a}_q^\dagger\hat{a}_q + g_q\hat{a}_q^\dagger\hat{a}_q(\hat{b}_q^\dagger + \hat{b}_q) + \Omega_q'(t)\hat{b}_q^\dagger\hat{b}_q + \varepsilon_q(\hat{a}_q^\dagger + \hat{a}_q), \tag{4}$$

where $\Omega_q'(t) = \Omega_q + g_1|\alpha_1(t)|^2$ is the effective resonant frequency of the mechanical mode $\hat{b}_q$ when taking into account its quadratic-coupling with the cavity mode $\alpha_1(t)$.

In the strong-driving regime, the quantum operators $\hat{a}_q$ and $\hat{b}_q$ can be written as

$$\hat{a}_q = \alpha_q + \hat{\tilde{a}}_q, \quad \hat{b}_q = \beta_q + \hat{\tilde{b}}_q, \tag{5}$$

where $\alpha_q = \langle\hat{a}_q\rangle$ ($\beta_q = \langle\hat{b}_q\rangle$) refers to the classical mean value and $\hat{\tilde{a}}_q$ ($\hat{\tilde{b}}_q$) the quantum fluctuating term of the cavity field $\hat{a}_q$ (the mechanical mode $\hat{b}_q$), respectively. By substituting Eq. (5) into Eq. (4), and omitting the classical terms,

we have the linearized Hamiltonian

$$\tilde{H}_{\rm eff} = \Delta'_q \hat{\tilde{a}}_q^\dagger \hat{\tilde{a}}_q + G_q(\hat{\tilde{a}}_q^\dagger + \hat{\tilde{a}}_q)(\hat{\tilde{b}}_q^\dagger + \hat{\tilde{b}}_q) + \Omega'_q(t)\hat{\tilde{b}}_q^\dagger \hat{\tilde{b}}_q, \tag{6}$$

where $\Delta'_q = \Delta_q - g_q(\langle \hat{b}_q^\dagger \rangle + \langle \hat{b}_q \rangle)$ is the modified detuning due to optomechanical coupling and $G_q = |\alpha_q| g_q$ is the linearized coupling strength.

Then we obtain the master equation from this linearized Hamiltonian

$$\rho = i[\rho, \tilde{H}_{\rm eff}] + \gamma \mathcal{D}[\hat{\tilde{a}}_q]\rho + \Gamma[n_{\rm th}(t) + 1]\mathcal{D}[\hat{\tilde{b}}_q]\rho + \Gamma n_{\rm th}(t)\mathcal{D}[\hat{\tilde{b}}_q^\dagger]\rho, \tag{7}$$

where $\mathcal{D}[\hat{o}]\rho = \hat{o}\rho\hat{o}^\dagger - (\hat{o}^\dagger\hat{o}\rho + \rho\hat{o}^\dagger\hat{o})/2$ is the Liouvillian in the Lindblad form for the operator $\hat{o}$, and $n_{\rm th}(t) = K_{\rm B}T/\hbar\Omega'_q(t)$ is the mean thermal phonon excitation number when the environmental temperature is $T$.

From this master equation, we can then obtain a group of closed differential equations for the second order terms

$$\frac{d\langle \hat{\tilde{b}}_q^\dagger \hat{\tilde{b}}_q \rangle}{dt} = -iG_q(-\langle \hat{\tilde{a}}_q^\dagger \hat{\tilde{b}}_q \rangle + \langle \hat{\tilde{a}}_q^\dagger \hat{\tilde{b}}_q \rangle^* + \langle \hat{\tilde{a}}_q \hat{\tilde{b}}_q \rangle^* - \langle \hat{\tilde{a}}_q \hat{\tilde{b}}_q \rangle) - \Gamma_q \langle \hat{\tilde{b}}_q^\dagger \hat{\tilde{b}}_q \rangle + \Gamma_q n_{\rm th}(t), \tag{8a}$$

$$\frac{d\langle \hat{\tilde{a}}_q^\dagger \hat{\tilde{a}}_q \rangle}{dt} = -iG_q(\langle \hat{\tilde{a}}_q^\dagger \hat{\tilde{b}}_q \rangle - \langle \hat{\tilde{a}}_q^\dagger \hat{\tilde{b}}_q \rangle^* + \langle \hat{\tilde{a}}_q \hat{\tilde{b}}_q \rangle^* - \langle \hat{\tilde{a}}_q \hat{\tilde{b}}_q \rangle) - \gamma_q \langle \hat{\tilde{a}}_q^\dagger \hat{\tilde{a}}_q \rangle, \tag{8b}$$

$$\frac{d\langle \hat{\tilde{a}}_q^\dagger \hat{\tilde{b}}_q \rangle}{dt} = -i[\Delta'_q + \Omega'_q(t)]\langle \hat{\tilde{a}}_q^\dagger \hat{\tilde{b}}_q \rangle - \frac{\gamma_q + \Gamma_q}{2}\langle \hat{\tilde{a}}_q^\dagger \hat{\tilde{b}}_q \rangle - iG_q(\langle \hat{\tilde{a}}_q^\dagger \hat{\tilde{a}}_q \rangle - \langle \hat{\tilde{b}}_q^\dagger \hat{\tilde{b}}_q \rangle + \langle \hat{\tilde{a}}_q^2 \rangle^* - \langle \hat{\tilde{b}}_q^2 \rangle), \tag{8c}$$

$$\frac{d\langle \hat{\tilde{a}}_q \hat{\tilde{b}}_q \rangle}{dt} = i[\Delta'_q - \Omega'_q(t)]\langle \hat{\tilde{a}}_q \hat{\tilde{b}}_q \rangle - \frac{\gamma_q + \Gamma_q}{2}\langle \hat{\tilde{a}}_q \hat{\tilde{b}}_q \rangle - iG_q(\langle \hat{\tilde{a}}_q^\dagger \hat{\tilde{a}}_q \rangle + \langle \hat{\tilde{b}}_q^\dagger \hat{\tilde{b}}_q \rangle + 1 + \langle \hat{\tilde{a}}_q^2 \rangle + \langle \hat{\tilde{b}}_q^2 \rangle), \tag{8d}$$

$$\frac{d\langle \hat{\tilde{a}}_q^2 \rangle}{dt} = (2i\Delta'_q - \gamma_q)\langle \hat{\tilde{a}}_q^2 \rangle - 2iG_q(\langle \hat{\tilde{a}}_q \hat{\tilde{b}}_q \rangle + \langle \hat{\tilde{a}}_q^\dagger \hat{\tilde{b}}_q \rangle^*), \tag{8e}$$

$$\frac{d\langle \hat{\tilde{b}}_q^2 \rangle}{dt} = [-2i\Omega'_q(t) - \Gamma_q]\langle \hat{\tilde{b}}_q^2 \rangle - 2iG_q(\langle \hat{\tilde{a}}_q \hat{\tilde{b}}_q \rangle + \langle \hat{\tilde{a}}_q^\dagger \hat{\tilde{b}}_q \rangle), \tag{8f}$$

where $\alpha_1(t)$ is the classical input, which is governed by the motion of equations shown in Eq. (3).

Our goal is to study the standard deviations $(\sigma_x, \sigma_p)$ of the quantum position and momentum $(\hat{x}, \hat{p})$ of the mechanical mode, which take the forms

$$\sigma_x = \sqrt{\langle \hat{x}^2 \rangle - \langle \hat{x} \rangle^2} \qquad \sigma_p = \sqrt{\langle \hat{p}^2 \rangle - \langle \hat{p} \rangle^2}. \tag{9}$$

Using the relations $\hat{x} = (\hat{b}_q + \hat{b}_q^\dagger)/\sqrt{2}$ and $\hat{p} = (\hat{b}_q - \hat{b}_q^\dagger)/\sqrt{2}i$, Eq. (9) can be rewritten as

$$\sigma_x = \frac{1}{\sqrt{2}}\sqrt{\langle (\hat{b}_q^\dagger)^2 \rangle + \langle \hat{b}_q^2 \rangle + \langle \hat{b}_q^\dagger \hat{b}_q \rangle + \langle \hat{b}_q \hat{b}_q^\dagger \rangle - \langle \hat{b}_q^\dagger \rangle^2 - \langle \hat{b}_q \rangle^2 - 2\langle \hat{b}_q \rangle \langle \hat{b}_q^\dagger \rangle}. \tag{10}$$

By replacing $b_q$ and $b_q^\dagger$ with the expressions $b_q = \langle b_q \rangle + \tilde{b}_q$ and $b_q^\dagger = \langle b_q^\dagger \rangle + \tilde{b}_q^\dagger$, we have the reduced form of $\sigma_x$

$$\sigma_x = \sqrt{\langle \hat{\tilde{b}}_q \hat{\tilde{b}}_q^\dagger \rangle + \langle \hat{\tilde{b}}_q^\dagger \hat{\tilde{b}}_q \rangle + \langle \hat{\tilde{b}}_q^2 \rangle + \langle (\hat{\tilde{b}}_q^\dagger)^2 \rangle} = \sqrt{\frac{1}{2} + \langle \hat{\tilde{b}}_q^\dagger \hat{\tilde{b}}_q \rangle + {\rm Re}[\langle \hat{\tilde{b}}_q^2 \rangle]}. \tag{11}$$

Therefore, the standard derivation $\sigma_x$ $(\sigma_p)$ is governed by both the classical part in Eq. (3) and the linearized quantum master equation in Eq. (8).

## ii. THE DYNAMICS OF THE QUANTUM MECHANICAL OSCILLATOR FOR DIFFERENT CLASSICAL INPUTS IN THE SETUP OF CONFIGURATION I.

We now show that the dynamics of the quantum mechanical resonator $\hat{b}_q$ is dominated by the classical controller $(\alpha_c,\ \beta_c)$. As shown in Figs. 2 (a), (d), and (g), we prepare the optomechanical system $(\alpha_c,\ \beta_c)$ in there periodic, multi-periodic, and chaotic regimes, by setting three different driving strengths, respectively. Then, we check the dynamics of the quantum mechanical resonator by reconstructing its generalized quantum orbit from the standard deviation $\sigma_x$. When the classical part is periodic [Fig. 2 (a)] and period-doubling [Fig. 2 (d)], the time series of the standard derivation $\sigma_x(t)$ [Figs. 2 (b) and (e)] and its generalized quantum orbits [Figs. 2 (c) and (f)] exhibit regular motions. When the classical optomechanical system is excited to a chaotic state [Fig. 2 (g)], the standard derivation $\sigma_x(t)$ in the quantum part corresponds to a chaotic motion [Fig. 2 (h)], and a chaotic attractor can be found in the generalized quantum orbit of the phase space [Fig. 2 (i)].

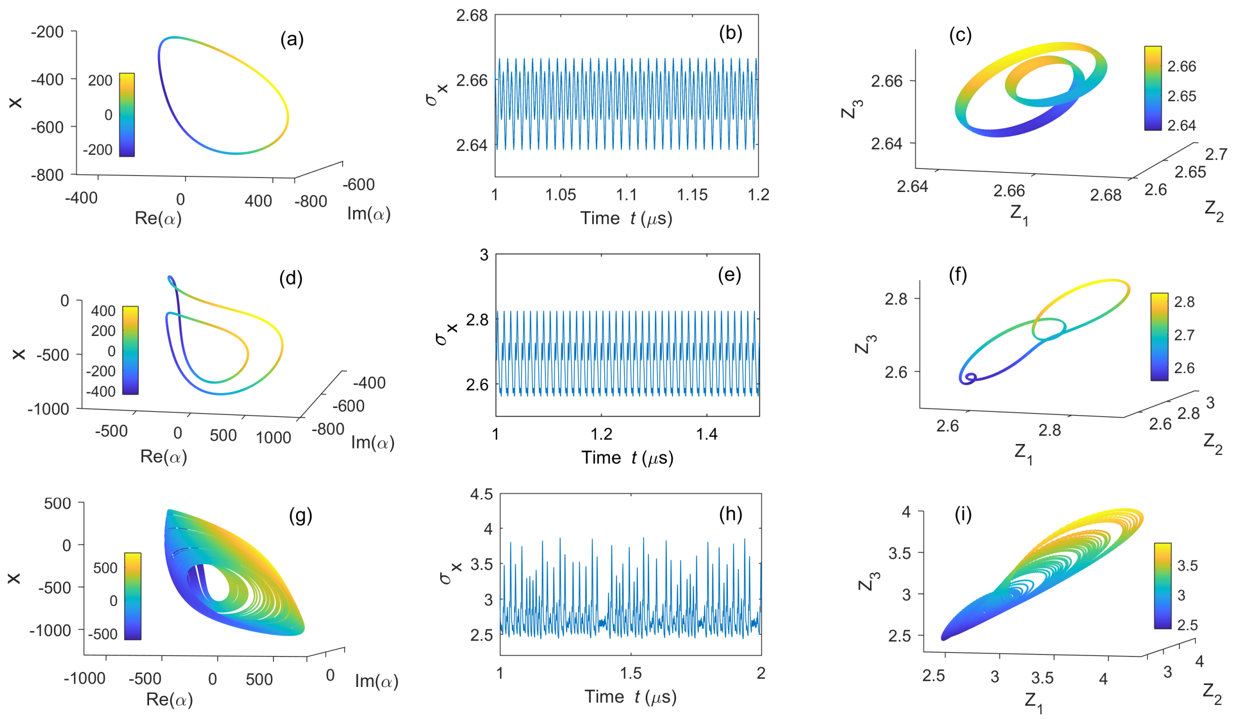


FIG. 2: (color online) The time series $\sigma_x(t)$ and its corresponding generalized quantum orbits, when the classical optomechanical system is set to be periodic, multi-periodic, and chaotic. The driving strength is $\varepsilon_s/\Omega = 370$ for (a), (b), and (c), $\varepsilon_s/\Omega = 400$ for (d), (e), and, (f), and $\varepsilon_s/\Omega = 433$ for (g), (h), and (i). Here, the time delay $\tau = 0.3$ ns. Other parameters are set as: $\Delta_c/\Omega_c = -1$, $\gamma_c/\Omega_c = 1$, $g_c/\Omega_c = 10^{-3}$, $\Gamma_c/\Omega_c = 2.8$, $\Omega_c/2\pi = 10^{-3}$, $\Delta_1/\Omega_q = 10^4$, $\gamma_1/\Omega_q = 6$, $\varepsilon_1/\Omega_c = 0$, $\Delta_q/\Omega_q = -2$, $\gamma_q/\Omega_q = 1$, $g_1/\Omega_q = 2$, $g_q'/\Omega_q = 10^{-3}$, $\Gamma_q/\Omega_q = 100$, $\Omega_q/2\pi = 0.01$ GHz, $k_{\mathrm{B}} = 1.38 \times 10^{-23}$ $\mathrm{m^2 kg \cdot s^{-2} K^{-1}}$, $\hbar = 1.0546 \times 10^{-34}$ $\mathrm{J \cdot s}$, and $T = 0.002$ K.

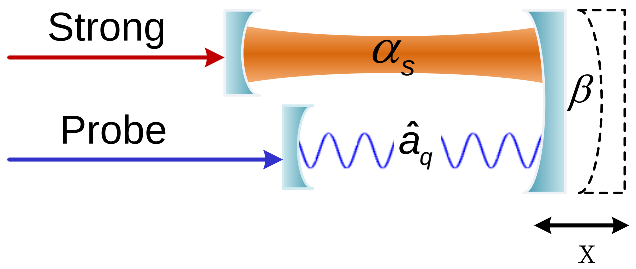


FIG. 3: (Color online) Schematic diagrams of an optomechanical setup for quantum chaos in configuration II. This setup includes a quantum cavity mode $\hat{a}_q$, a classical cavity mode $\alpha_s$, and a classical mechanical mode $\beta$. Both the quantum cavity $\hat{a}_q$ and the classical cavity $\alpha_s$ are coupled to the mechanical mode $\beta$, and the coupling strengths are $g_s$ and $g_q$, respectively.

## iii. THE DYNAMICS OF THE QUANTUM CAVITY FOR DIFFERENT CLASSICAL INPUTS IN CONFIGURATION II

We use the quantum master equation to study the dynamics of this quantum cavity in Fig. (3). The density matrix takes the form $\rho = \sum_{j,k=0}^{2} \lambda_{j,k} |j\rangle\langle k|$, where $\sum_{j=0}^{2} \lambda_{j,j} = 1$. Here, $\rho$ is governed by the system master equation

$$\rho = i[\rho, H_{\mathrm{eff}}(t)] + \gamma_q \mathcal{D}[\hat{a}_q]\rho \tag{12}$$

where $\mathcal{D}[\hat{a}_q]\rho = \hat{a}_q \rho \hat{a}_q^\dagger - (\hat{a}_q^\dagger \hat{a}_q \rho + \rho \hat{a}_q^\dagger \hat{a}_q)/2$ is the Liouvillian in the Lindblad form for $\hat{a}_q$.

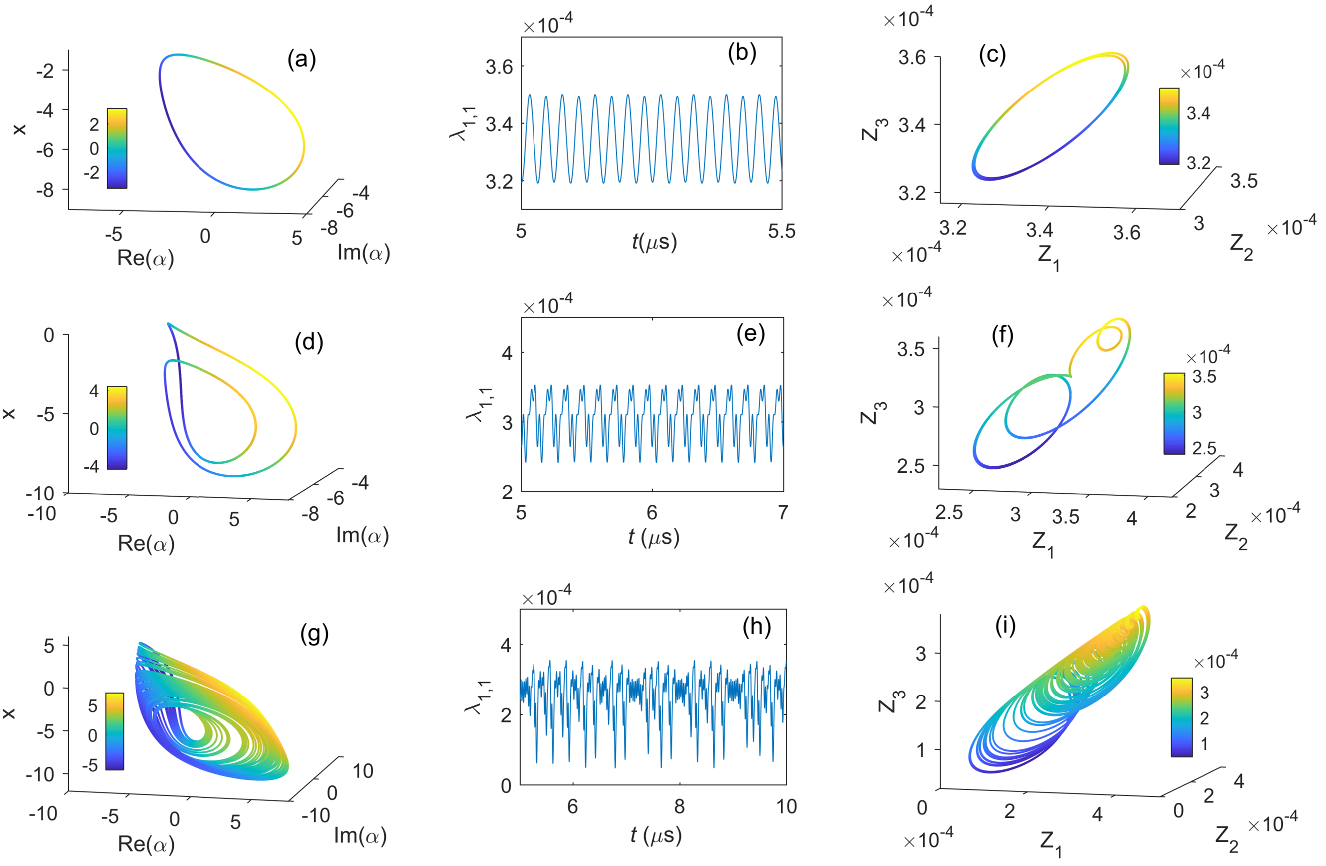


FIG. 4: (color online) The dynamics of the quantum cavity $\hat{a}_q$ when the classical controllers in different regimes. The phase portraits of the classical optomechanical controller ($\alpha_s$,$\beta$) when it is prepared to be (a) periodic, (d) multi-periodic, and (g) chaotic. Correspondingly, the time evolutions of $\lambda_{1,1}(t)$ for the quantum cavity $\hat{a}_q$ are shown in (b), (e), and (h), which lead to the generalized quantum orbits [(c), (f), and (i)] , respectively. The driving strength is set to be $\varepsilon_s/\Omega = 3.87$ for (a), (b), and (c), $\varepsilon_s/\Omega = 4$ for (d), (e), and, (f), and $\varepsilon_s/\Omega = 4.33$ for (g), (h), and (i). Here, the time delay $\tau = 2$ ns for (c), $\tau = 3$ ns for (f), and $\tau = 4$ ns for (i). Other parameters are: $\Delta_s/\Omega = -1$, $g_s/\Omega = g_q/\Omega = 0.1$, $\gamma_s/\Omega = 1$, $\gamma_0/\Omega = 0.95$, $\Delta_q/\Omega = 1$, $\varepsilon_q/\Omega = 0.01$, $\Gamma/\Omega = 10^{-3}$, and $\Omega/2\pi = 0.1$ GHz.

We study the dynamics of the quantum cavity $\hat{a}_q$ for different classical inputs. In this section, the classical optomechanical system is adjusted to be periodic [Fig. 4 (a)], 2-periodic [Fig. 4 (d)], and chaotic [Fig. 4 (g)]. It can be seen that the evolution of the quantum cavity is dominated by the classical optomechanical system. When the classical optomechanical system is periodic and 2-periodic, the quantum cavity is also in regular motions. While, a chaotic attractor appears in the generalized quantum orbit [Fig. 4 (i)] when this classical controller is chaotic [Fig. 4 (g)]. Here, $\lambda_{1,1}(t)$ is numerically calculated from the master equation. The generalized quantum orbit of this quantum cavity is obtained by embedding the time-delayed coordinates $\lambda_{1,1}(t_0)$, $\lambda_{1,1}(\tau)$, $\lambda_{1,1}(2\tau)$, ..., $\lambda_{1,1}(N\tau)$ into a 4D phase space.

## iv. NONLINEARITY OF CLOSED QUANTUM SYSTEMS IN CONFIGURATION II

In this section, we first provide the definition of linearity for a closed quantum system. A quantum system $|\psi\rangle$ in $N$ possible quantum states ($|\phi_1\rangle$, $|\phi_2\rangle$, ..., $|\phi_N\rangle$) can be represented as: $|\psi\rangle = \sum_{k=1}^{N} p_k|\phi_k\rangle$, where $p_k$ denotes the probability amplitude of the $k$-th quantum state $\phi_k$. Here, the quantum state $|\psi\rangle$ is governed by the Schrodinger equation

$$i\frac{d|\psi\rangle}{dt} = H|\psi\rangle, \tag{13}$$

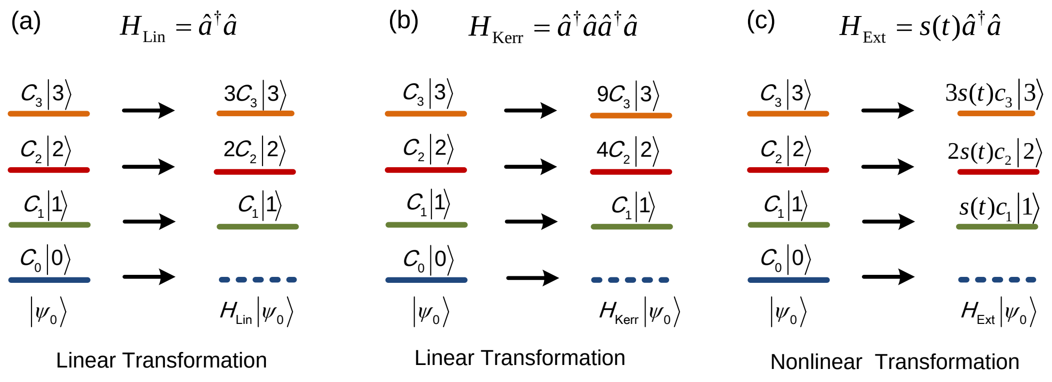


FIG. 5: (color online) The probability distributions of a four energy level quantum state $|\psi\rangle$ when three different Hamiltonians act on that state. (a) A linear cavity: $H_{\rm Lin} = \hat{a}^\dagger\hat{a}$, (b) a Kerr cavity: $H_{\rm Kerr} = \hat{a}^\dagger\hat{a}\hat{a}^\dagger\hat{a}$, and (c) a classical-system-assistant quantum system: $H_{\rm Ext} = s(t)\hat{a}^\dagger\hat{a}$, where $s(t)$ is an external classical signal and the input quantum state takes the form: $|\psi_0\rangle = c_0|0\rangle + c_1|1\rangle + c_2|2\rangle + c_3|3\rangle$.

where $H$ is the Hamiltonian of the quantum system. By substituting $|\psi\rangle = \sum_{k=1}^{N} p_k|\phi_k\rangle$ into Eq. (1) and combining the coefficients of the same quantum states, we have the differential equation

$$\dot{\mathbf{p}} = \mathbf{F}(\mathbf{p}), \tag{14}$$

where $\mathbf{p}$ denotes the vector of the probability amplitudes: $\mathbf{p} = (p_0, p_1, ..., p_n)'$, and $\mathbf{F}$ denotes the function of the $N$-dimensional $\mathbf{p}$.

*Definition 1.* A function $\mathbf{F}$ is nonlinear if it satisfies

$$\mathbf{F}(Ap_i + Bp_j) \neq A\mathbf{F}(p_i) + B\mathbf{F}(p_j), \quad p_i, p_j \in \mathbf{p} \tag{15}$$

for arbitrary $p_i$ and $p_j$ in the domain $\mathbf{p}$, and all scales $A$ and $B$.

It was usually thought that a quantum system is nonlinear if its Hamiltonian contains high-order harmonic terms (above two orders). For instance, a quantum linear cavity ($H_{\rm Lin} = \hat{a}^\dagger\hat{a}$) is considered as a linear system, while a quantum Kerr cavity ($H_{\rm Kerr} = \hat{a}^\dagger\hat{a}\hat{a}^\dagger\hat{a}$) is treated as a typical nonlinear system. Here, we list three typical quantum devices, and check their linearity according to definition 1.

Figure 5 shows the changes of a quantum state $|\psi_0\rangle$ with coupling to three different quantum devices: a linear cavity $H_{\rm Lin}$ [Fig. 5(a)], a Kerr cavity $H_{\rm Kerr}$ [Fig. 5(b)], and a linear cavity driven by an external classical signal $H_{\rm Ext}$ [Fig. 5(c)]. In the weak-driving limit, the initial input state $|\psi_0\rangle$ can be limited to a four energy level system: $|\psi_0\rangle = \Sigma_{j=0}^{3} c_j|j\rangle$, where $c_j$ represents the probability amplitude of the state $|j\rangle$. The left parts and the right parts of Figs. 5(a), (b), and (c) show the energy level distributions of a quantum state $|\psi_0\rangle$ without and with three different Hamiltonians acting on.

As shown in Fig. 5(a), a linear cavity changes the probability amplitude of each energy level of the quantum state $|\psi_0\rangle$ in a linear way, which coincides with previous studies. One surprising result is that the Kerr cavity does not generate any nonlinearity term when its Hamiltonian $H_{\rm Kerr}$ acts on $|\psi_0\rangle$ [Fig. 5(b)]. It just excites photons to the higher energy levels when compared to the linear cavity. It can be easily concluded that an isolated non-time-delay quantum system with time-independent Hamiltonian is linear in the sense of configuration I.

In Fig. 5(c), we consider a quantum system driven by a external classical signal $s(t)$ with the interaction Hamiltonian $H_{\rm Ext} = s(t)\hat{a}^\dagger\hat{a}$. Here, $s(t)$ is output by a classical system: $\dot{\mathbf{q}} = \mathbf{G}(\mathbf{q})$, where $\mathbf{G}$ is the function of $\mathbf{q}$, where $\mathbf{q} = (q_0, ..., q_n, s)$. When $s(t) \neq$ constant, nonlinear terms such as $s(t)c_1$ emerge in the quantum system. In this case, we consider a larger state space of the whole system, including the quantum and the classical parts: $\mathbf{c}_T = \mathbf{c} \bigoplus \mathbf{q}$. It can be seen that the linearity of a quantum system is changed by coupling to a classical system. To summarize, a quantum system shown in Fig. 5(c) can be converted from linear to nonlinear regimes by coupling to a classical system.

### A. The dynamics of a closed quantum cavity for different classical inputs in configuration II

In this section, we check the relationship between the classical controller and a closed quantum cavity. Note that in closed quantum systems, we construct generalized quantum orbits in a different way. The setup is also shown in

Fig. 3(a), a quantum cavity $\hat{a}_q$ and a classical cavity $\alpha_s$ are coupled to the same classical mechanical mode $\beta$. Here, the classical cavity $\alpha_s$ is strongly driven to chaos, and this chaos can be transferred to the quantum cavity $\hat{a}_q$ through the classical mechanical mode. The Hamiltonian of the total system reads

$$H_{\mathrm{eff}} = \Delta_q \hat{a}_q^\dagger \hat{a}_q + 2g_q x(t)\hat{a}_q^\dagger \hat{a}_q, \tag{16}$$

where $\Delta_q$ is the detuning of $\hat{a}_q$, $x(t) = (\beta + \beta^*)/2$ is the mechanical displacement of the classical mechanical mode $\beta$, and $g_q$ is the coupling strength between $\hat{a}_q$ and $x(t)$.

First, we focus on the classical components $(\alpha_s, \beta)$, their equations of motion are given by

$$\dot{\alpha}_s = -i\Delta_s\alpha_s - \frac{\gamma_s}{2}\alpha_s - ig_s\alpha_s(\beta+\beta^*) - i\varepsilon_s\ , \tag{17a}$$

$$\dot{\beta} = \left(-i\Omega - \frac{\Gamma}{2}\right)\beta - ig_s|\alpha|^2\ , \tag{17b}$$

Let $x = \frac{1}{2}(\beta+\beta^*)$ and $p = \frac{1}{2i}(\beta-\beta^*)$, then Eq. (17) can be rewritten in a 4-dimensional space

$$\frac{dx}{dt} = -\frac{\Gamma}{2}x + \Omega p, \tag{18a}$$

$$\frac{dp}{dt} = -\frac{\Gamma}{2}p - \Omega x - g_s|\alpha|^2, \tag{18b}$$

$$\frac{d\mathrm{Re}(\alpha_s)}{dt} = -(\Delta_s - 2g_s x)\mathrm{Im}(\alpha_s) - \frac{\gamma_s}{2}\mathrm{Re}(\alpha_s), \tag{18c}$$

$$\frac{d\mathrm{Im}(\alpha_s)}{dt} = (\Delta_s - 2g_s x)\mathrm{Re}(\alpha_s) - \frac{\gamma_s}{2}\mathrm{Im}(\alpha_s) - \varepsilon_s, \tag{18d}$$

where $\Delta_s$, $\gamma_s$, and $\varepsilon_s$ refer to the detuning, damping rate, and driving strength of the classical cavity mode $\alpha_s$; while $\Omega$ and $\Gamma$ are the resonance frequency and the damping rate of the mechanical mode $\beta$; and $g_s$ is the coupling strength between the classical cavity $\alpha_s$ and mechanical modes $\beta$.

Then, we now move to the quantum part of this setup. In the Schrodinger picture, the quantum cavity $\hat{a}_q$ can be represented in the Fock space: $|\psi_{a_q}\rangle = \Sigma_{k=0}^{\infty} c_k|k\rangle$, where $c_k$ is the probability amplitude of the $k$-th energy level. In the weak-driving limit, the infinite dimensional quantum harmonic oscillator $|\psi_{a_q}\rangle$ can be reduced to a three energy level quantum system: $|\psi_{a_q}\rangle = c_0|0\rangle + c_1|1\rangle + c_2|2\rangle$, where $c_0 \approx 1$. By combining the coefficients of the same energy level term $|k\rangle$ $(k = 0, 1, 2)$ in the Schrodinger equation, we have the equations of the probability amplitudes $c_1$ and $c_2$,

$$\dot{c}_1 = -i[\Delta_q + s(t)]c_1 - \frac{\gamma_0}{2}c_1 + i\varepsilon_q(1 + c_2), \tag{19a}$$

$$\dot{c}_2 = -i[2\Delta_q + s(t)]c_2 - \frac{\gamma_0}{2}c_2 + \sqrt{2}i\varepsilon_q c_1, \tag{19b}$$

where $\gamma_0$ and $\varepsilon_q$ are the corresponding damping rate and driving strength of the quantum cavity mode $\hat{a}_q$, respectively. Here, $(c_1, c_2)$ can be expanded into a 4-dimensional real phase space $[\mathrm{Re}(c_1), \mathrm{Im}(c_1), \mathrm{Re}(c_2), \mathrm{Im}(c_2)]$, and thus, Eq. (19) can be rewritten as

$$\frac{d\mathrm{Re}(c_1)}{dt} = -\frac{\gamma_0}{2}\mathrm{Re}(c_1) + [\varepsilon_q + \Delta_q + 2g_q x(t)]\mathrm{Im}(c_1), \tag{20a}$$

$$\frac{d\mathrm{Im}(c_1)}{dt} = -[\varepsilon_q + \Delta_q + 2g_q x(t)]\mathrm{Re}(c_1) - \frac{\gamma_0}{2}\mathrm{Im}(c_1) + \varepsilon_q, \tag{20b}$$

$$\frac{d\mathrm{Re}(c_2)}{dt} = -\frac{\gamma_0}{2}\mathrm{Re}(c_2) + [\Delta_q + 2g_q x(t)]\mathrm{Im}(c_2) - \varepsilon_q\mathrm{Im}(c_1), \tag{20c}$$

$$\frac{d\mathrm{Im}(c_2)}{dt} = -[\Delta_q + 2g_q x(t)]\mathrm{Re}(c_2) - \frac{\gamma_0}{2}\mathrm{Im}(c_2) + \varepsilon_q\mathrm{Re}(c_1), \tag{20d}$$

We perform numerical simulations for the classical parts ($\alpha_s$, $\beta$) in Eq. (18) and the quantum component $\hat{a}_q$ in Eq. (20). Here, the generalized quantum orbits are constructed by [Re($c_1$), Im($c_1$), Re($c_2$), Im($c_2$)]. Figures 6(a), (c), and (e) illustrate the phase portraits of the classical optomechanical system when it is prepared to period [Fig. 6(a)], period doubling [Fig. 6(c)], and chaos [Fig. 6(e)]. The corresponding generalized quantum orbits are shown in Figs. 6(b), (d), and (f). As shown in Figs. 6(a) and (b), the classical optomechanical system in the periodic

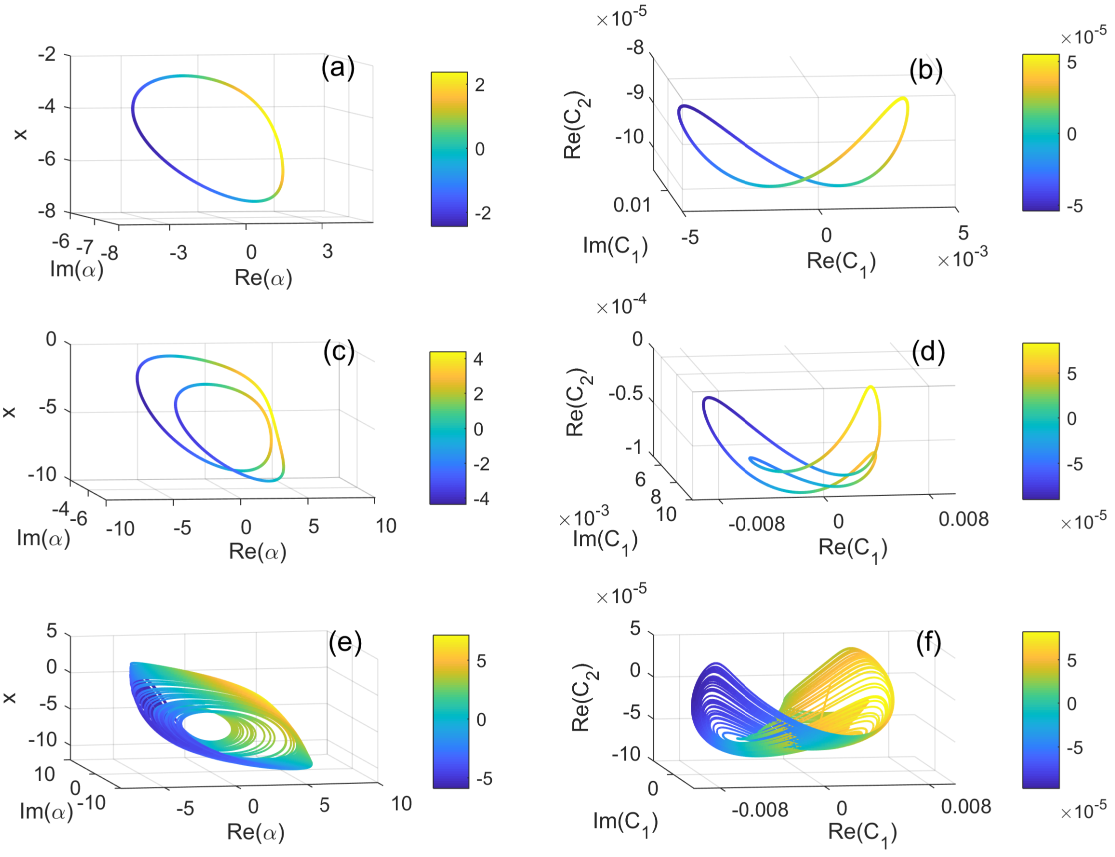


FIG. 6: (color online) Phase portraits for the classical and quantum components, when the driving strength $\varepsilon_s/\Omega = 3.7$ for (a) and (b), $\varepsilon_s/\Omega = 4$ for (c) and (d), and $\varepsilon_s/\Omega = 4.33$ for (e) and (f). In (a), (c), and (e), the fourth component $p$ of the classical optomechanical system is characterized by the quantified gradually changing colors. Analogously, $\mathrm{Im}(c_2)$ is the fourth variable in (b), (d), and (f). Other parameters are the same in Fig. 4.

regime drives the quantum cavity mode to be periodic [Figs. 6(a)], i.e., a limit circle is shown both in the quantum generalized orbit [Figs. 6(b)]. When increasing the driving strength to $\varepsilon_s/\Omega = 4$, the classical optomechanical system transits from period to period doubling [See Fig. 4(c)], which drives the quantum cavity to period doubling as well [See Fig. 6(d)]. When the classical system is in chaotic regime [See Fig. 6(e)], the quantum part characterized by $\mathbf{c}$ is also driven to be chaotic, i.e, a chaotic attractor is shown in Fig. 6(f). Moreover, as a indicator of chaos, the largest Lyapunov exponent is calculated to be positive. We find that quantum chaos is also achievable in a closed quantum cavity.
